# Supplementary material for: IC-Portrait: In-Context Matching for View-Consistent Personalized Portrait
Source: arXiv:2501.17159 source file (2025-01-31)
Supplement: Supplementary file 1 [file appendix.tex]

\chapter{Dummy Appendix}

You can defer lengthy calculations that would otherwise only interrupt
the flow of your thesis to an appendix.
